# Supplementary material for: Dispersed Exponential Family Mixture VAEs for Interpretable Text Generation
Source: arXiv:1906.06719 source file (2020-08-21)
Supplement: Supplementary file 1 [file appendix.tex]

\section{Proof of Mode Collapse}

The probability density function of the $c$-th component of mixture priors could be defined by its natural parameters $\eta_c$ according to the definition of exponential family:
\begin{equation*}
    p_{\eta}(z|c) = \exp (<\eta_c, \phi(z)> - A(\eta_c)),
\end{equation*}
in which $\phi=[\phi_1, \phi_2, ..., \phi_D]$ is a vector of functions of $z$ called sufficient statistics. For example, the sufficient statistics of normal distribution is $[z,z^2]$. For each sufficient statistic $\phi_d$, there is a corresponding natural parameter $\eta_d$. $<\eta, \phi(z)>$ is the inner-product of vector $\eta$ and $\phi$. $A(\eta_c)$ is the log-partition function, which is a function of natural parameters $\eta_c$.

Considering the $\regz$ term in $\ELBO$:
\begin{equation}
\begin{aligned}
     \E_{q_\phi(c|x)} & \E_{q_\phi(z|x)}\log \frac{p_\eta(z|c)}{q_\phi(z|x)}=\\
    & \E_{q_\phi(z|x)} [ \E_{q_\phi(c|x)}\log p_\eta(z|c) ] - \E_{q_\phi(z|x)}\log q_\phi(z|x).
\end{aligned}
\end{equation}
In terms of the probability density function of exponential family, $\E_{q_\phi(c|x)}\log p_\eta(z|c)$ could be re-written as
\begin{equation}
\begin{aligned}
    \E_{q_\phi(c|x)}\log \exp(<\eta_c, \phi(x)> - A(\eta_c))  \\
    = <\E_{q_\phi(c|x)} \eta_c, \phi(x)> - \E_{q_\phi(c|x)} A(\eta_c)
\end{aligned}
\end{equation}

Define the weighted expectation of natural parameters $\E_{q_\phi(c|x)}\eta_c$ as $\overline{\eta}$. Then,
\begin{equation}
\begin{split}
& \E_{q_\phi(c|x)}\log p_\eta(z|c)  \\
& = <\overline{\eta}, \phi(x)> - A(\overline{\eta}) - (\E_{q_\phi(c|x)} A(\eta_c) - A(\overline{\eta}))
\\ & = \log \hat{p}_{\overline{\eta}}(z|x) - (\E_{q_\phi(c|x)} A(\eta_c) - A(\E_{q_\phi(c|x)} \eta_c)),
\end{split}
\end{equation}
in which $\hat{p}_{\overline{\eta}}(z|x)=\exp{(<\overline{\eta}, \phi(x)> - A(\overline{\eta}))}$.  $\hat{p}_{\overline{\eta}}(z|x)$ is a distribution with the same sufficient statistics as priors but different parameters $\overline{\eta}$. Noted that the feasible domain of exponential family is a convex set, thus $\overline{\eta}$ is a feasible natural parameter as well.

As a result, the $\regz$ could be re-written as an ``average'' KL divergence term of $z$ and a dispersion term with respect to priors parameters and $q_\phi(c|x)$,
\begin{equation}
\begin{split}
    \E_{q_\phi(z|x)} & \sum_{c}q_\phi(c|x)\log \frac{p_\eta(z|c)}{q_\phi(z|x)}= \\ 
   & \underbrace{-\KL(q_\phi(z|x)||\hat{p}_\eta(z|x))}_\text{Average $\mathcal{R}_z$} \\
   &- \underbrace{(\E_{q_\phi(c|x)}A(\eta_c) - A(\E_{q_\phi(c|x)}\eta_c))}_\text{Dispersion term $\LL_d$}.
\end{split}
\end{equation}

We further analyze the relationship between dispersion term $\LL_d$ and the degree of dispersion of prior parameters. Firstly, we define the a weighted variance of natural parameters as the trace of variance matrix of natural parameters:
\begin{equation}
\begin{aligned}
    \text{Var}_{q(c|x)} \eta_c & = \text{Tr} \Big{(} \E_{q(c|x)} [ (\eta_c - \E_{q(c|x)}\eta_c)^T(\eta_c - \E_{q(c|x)}\eta_c) ] \Big{)}, \\
    & = \sum_d \E_{q(c|x)} (\eta_c^d)^2 - (\E_{q(c|x)} \eta_c^d)^2.
\end{aligned}
\end{equation}
in which $\eta_c^d$ is the $d$-th dimension of $\eta_c$. The weighted variance term reflects the discrepancy between parameters of priors under distribution $q(c|x)$.
If we calculate the gradient of this variance term  with respect to $\eta_c$:
\begin{equation}
\begin{split}
\nabla_{\eta_c} \text{Var}_{q(c|x)}\eta_c = 2 q(c|x) (\eta_c - (E_{q(c|x)}\eta_c)).
\end{split}
\end{equation}
In the meantime, we calculate the gradient of dispersion term $\LL_d$ with respect to $\eta_c$: 
\begin{equation}
\begin{split}
\nabla_{\eta_c} \LL_d = q(c|x) ( \nabla A|_{\eta_c} -  \nabla A|_{E_{q(c|x)}\eta_c} )
\end{split}
\end{equation}
Noted that the log-partition function $A$ is convex. It has $(\nabla A|x - \nabla A|y)(x-y)\geq 0$.
As a result, we have
\begin{equation} \label{eq: proof_of_gradient}
    ( \nabla_{\eta_c} \LL_d)^T  \cdot (  \nabla_{\eta_c} \text{Var}_{q(c|x)} \eta_c ) \geq 0.
\end{equation}
When $A$ is strictly convex, the dispersion term is larger than zero and inner product of gradients in Eq.~\ref{eq: proof_of_gradient} is larger than zero as well. 
If the gradient descent methods are used for optimizing the $\ELBO$, it will implicitly minimizing the weighted variance of prior parameters when mining the $\LL_d$.

\begin{figure}[tb]
    \subfloat[$q(c=1|x)=0.5$]{
     \centering
     % \vspace{-20 pt}
     \includegraphics[scale=0.28]{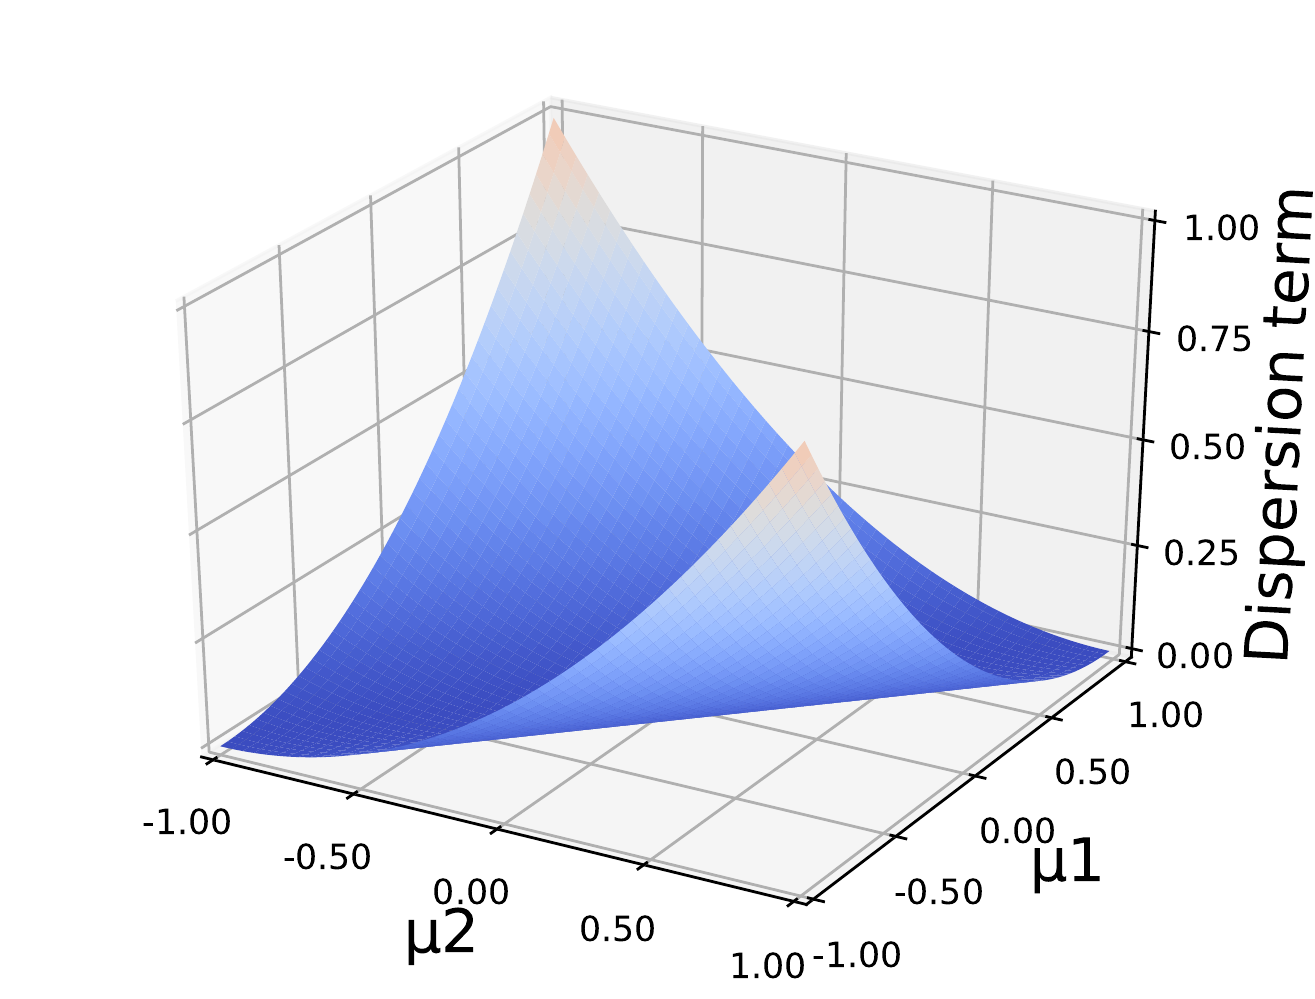}
      \hspace {3 pt}
     }
     \subfloat[$q(c=1|x)=0.2$]{
      \hspace {3 pt}
     \centering
     \includegraphics[scale=0.28]{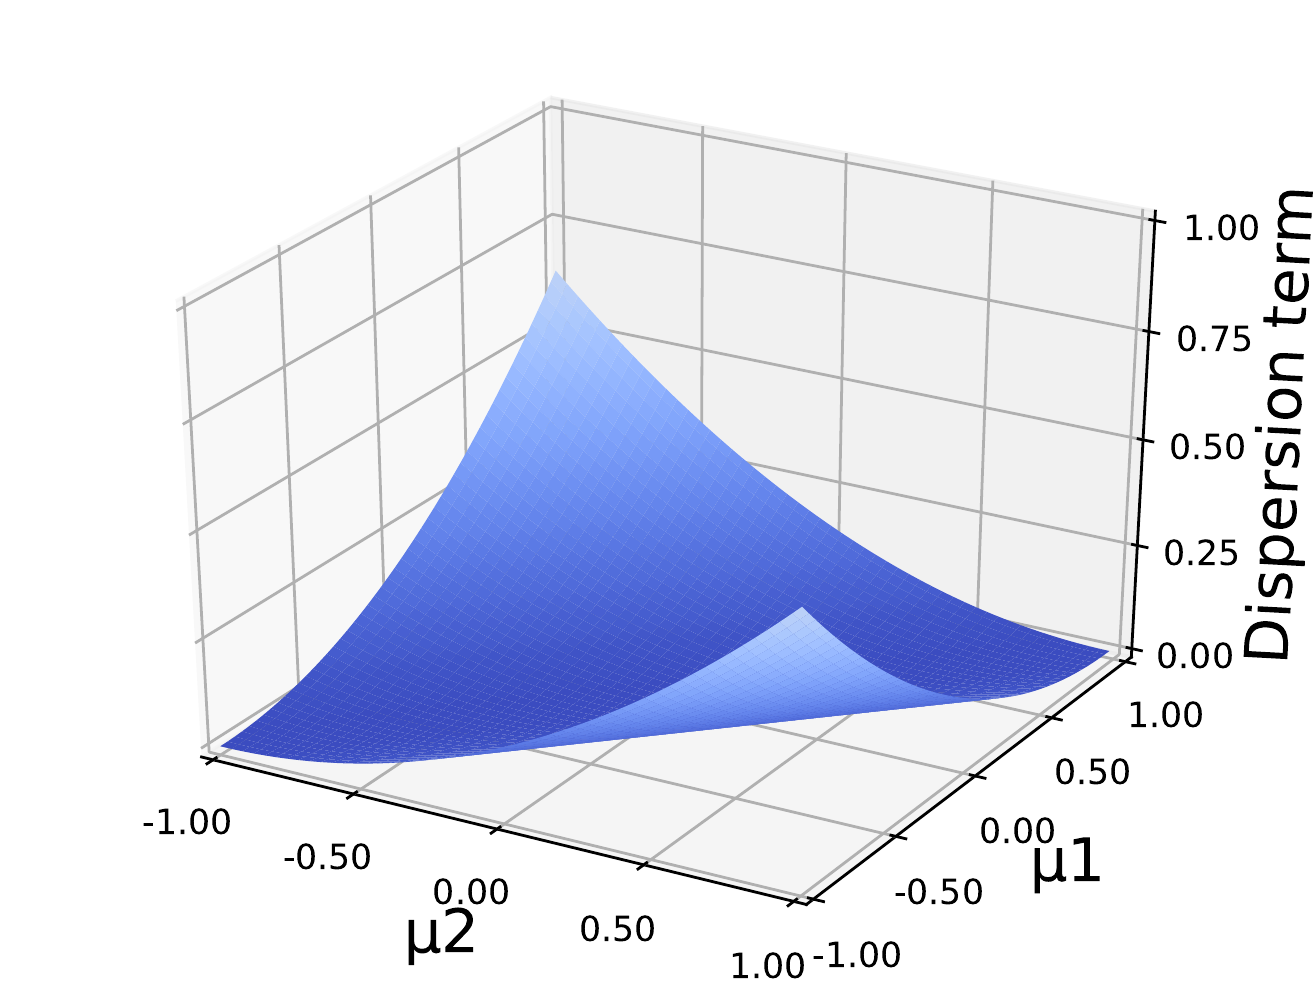}
       \hspace {3 pt}
     }
      \vspace{-6 pt}
    \caption{Dispersion term $\LL_d$ of GMVAE with respect to the parameters of two prior components under different posterior $q(c|x)$.}
    \label{fig:gaussian_dispersion}
\end{figure}

It should be noticed that the variance of prior parameters are weighted by posterior distribution $q_\phi(c|x)$. 
The dispersion terms of two-Gaussian mixture priors under different posterior distribution are shown in Fig~\ref{fig:gaussian_dispersion}. 
Under an unbalanced posterior distribution $q_\phi(c|x)$, the dispersion term is smaller in general, although it still takes the minimum value ($=0$) when parameters of all components are equal.
If $x$ corresponds to a certain $c$, which means the $q_\phi(c|x)$ has a one-hot probability mass function, both the dispersion term and variance term come to zero. Therefore, the mutual information is helpful to alleviate the mode-collapse as well because it implicitly enhances the correspondence between $x$ and $c$.

\section{Hyper-Parameters}
\label{appendix: hyper}
Bidirectional GRU encoder and one-layer GRU decoder with 512 hidden units are adopted. The size of word embedding is set as 512. Sentence longer than 40 will be cut off. Vocabulary size is set to 10,000. Latent variable $z$ is concatenated with input word embedding at each decoding step. 
Adam optimizer is adopted with learning rate of 0.001. Batch size is set to 30. 
During training of all VAE models, we sample the latent variable $z$ from posterior $q_\phi(z|x)$ for 20 times, and average their the reconstruction loss.
All results were obtained by repeating the experiment three times and taking an average.

We also illustrate how $\beta$ will affect the model performance in Fig.~\ref{fig:ptb_beta}; and we generally find that larger $\beta$ can get better results. % As a result, we use $\beta=0.8$ for experiment in PTB and DD.

\begin{figure}[tb]
    \centering
    \includegraphics[scale=0.3]{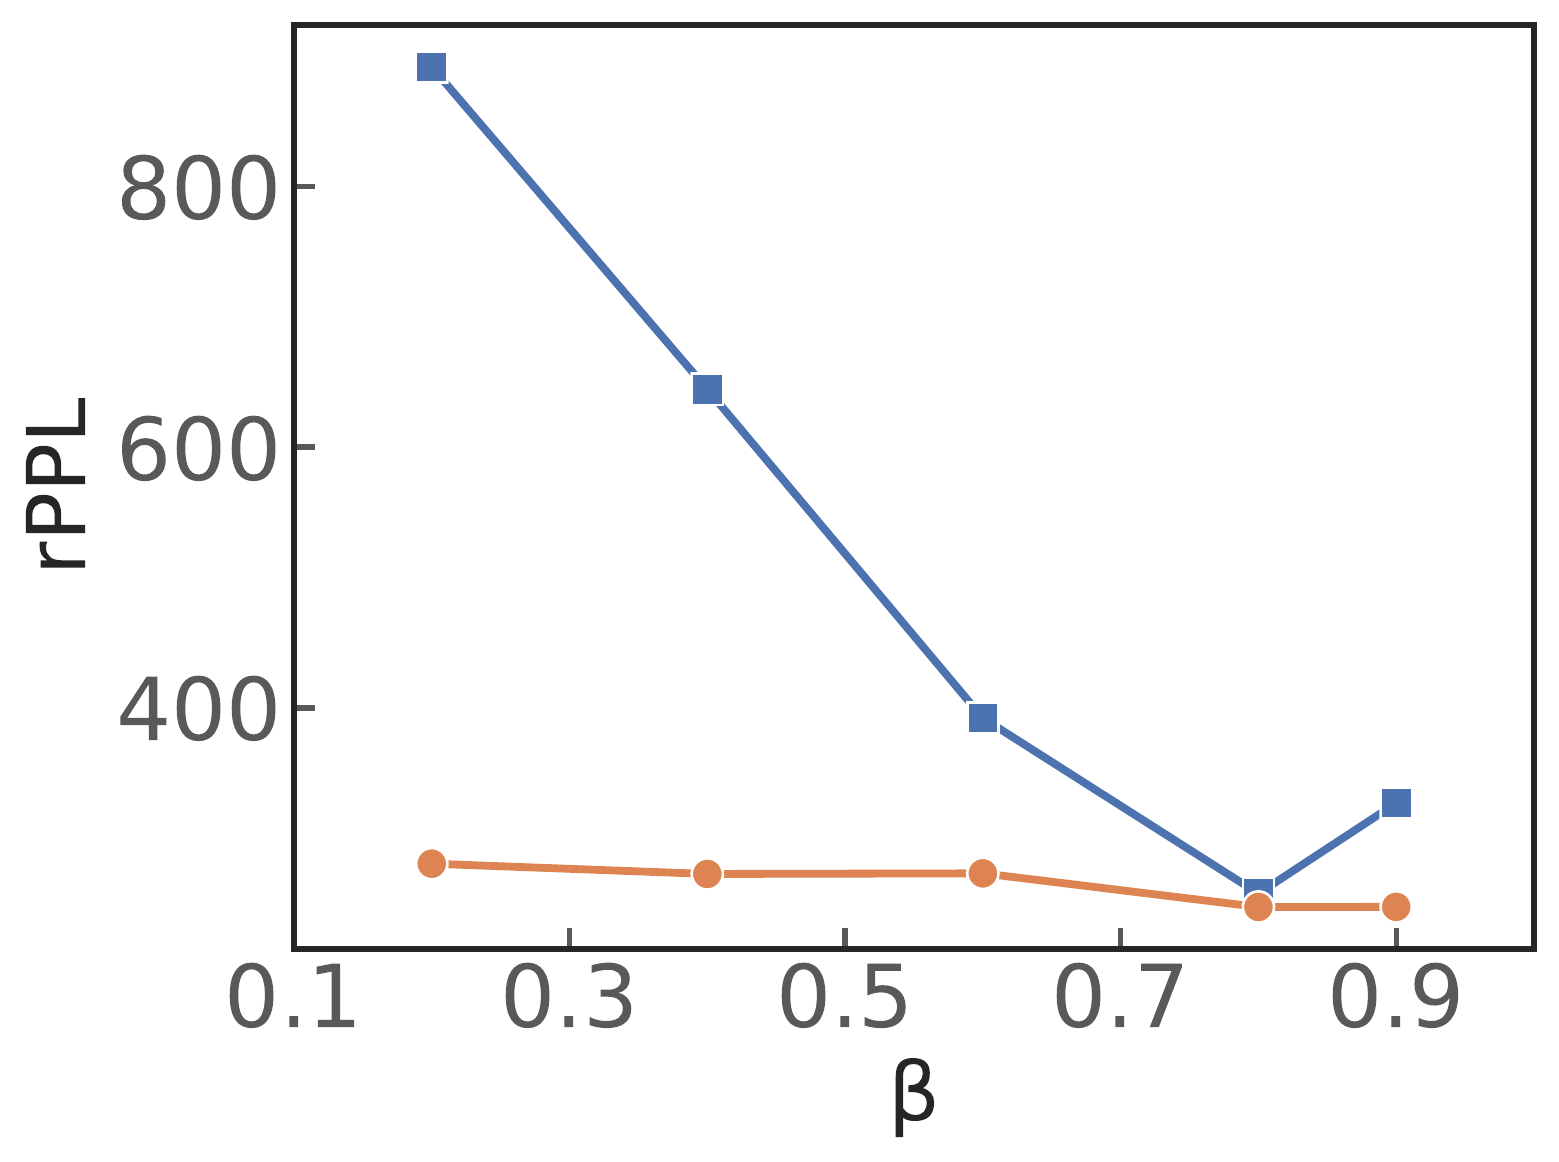}
    \caption{Reverse perplexity (rPPL) of \methodshort with different $\beta$, on the validation set of PTB. Results of \methodshort and \methodshort $+$ $\LL_{\text{mi}}$ are displayed by the blue lines and orange lines, respectively.}
    \label{fig:ptb_beta}
\end{figure}
% \begin{figure}[tb]
%     \centering
%     \includegraphics[scale=0.3]{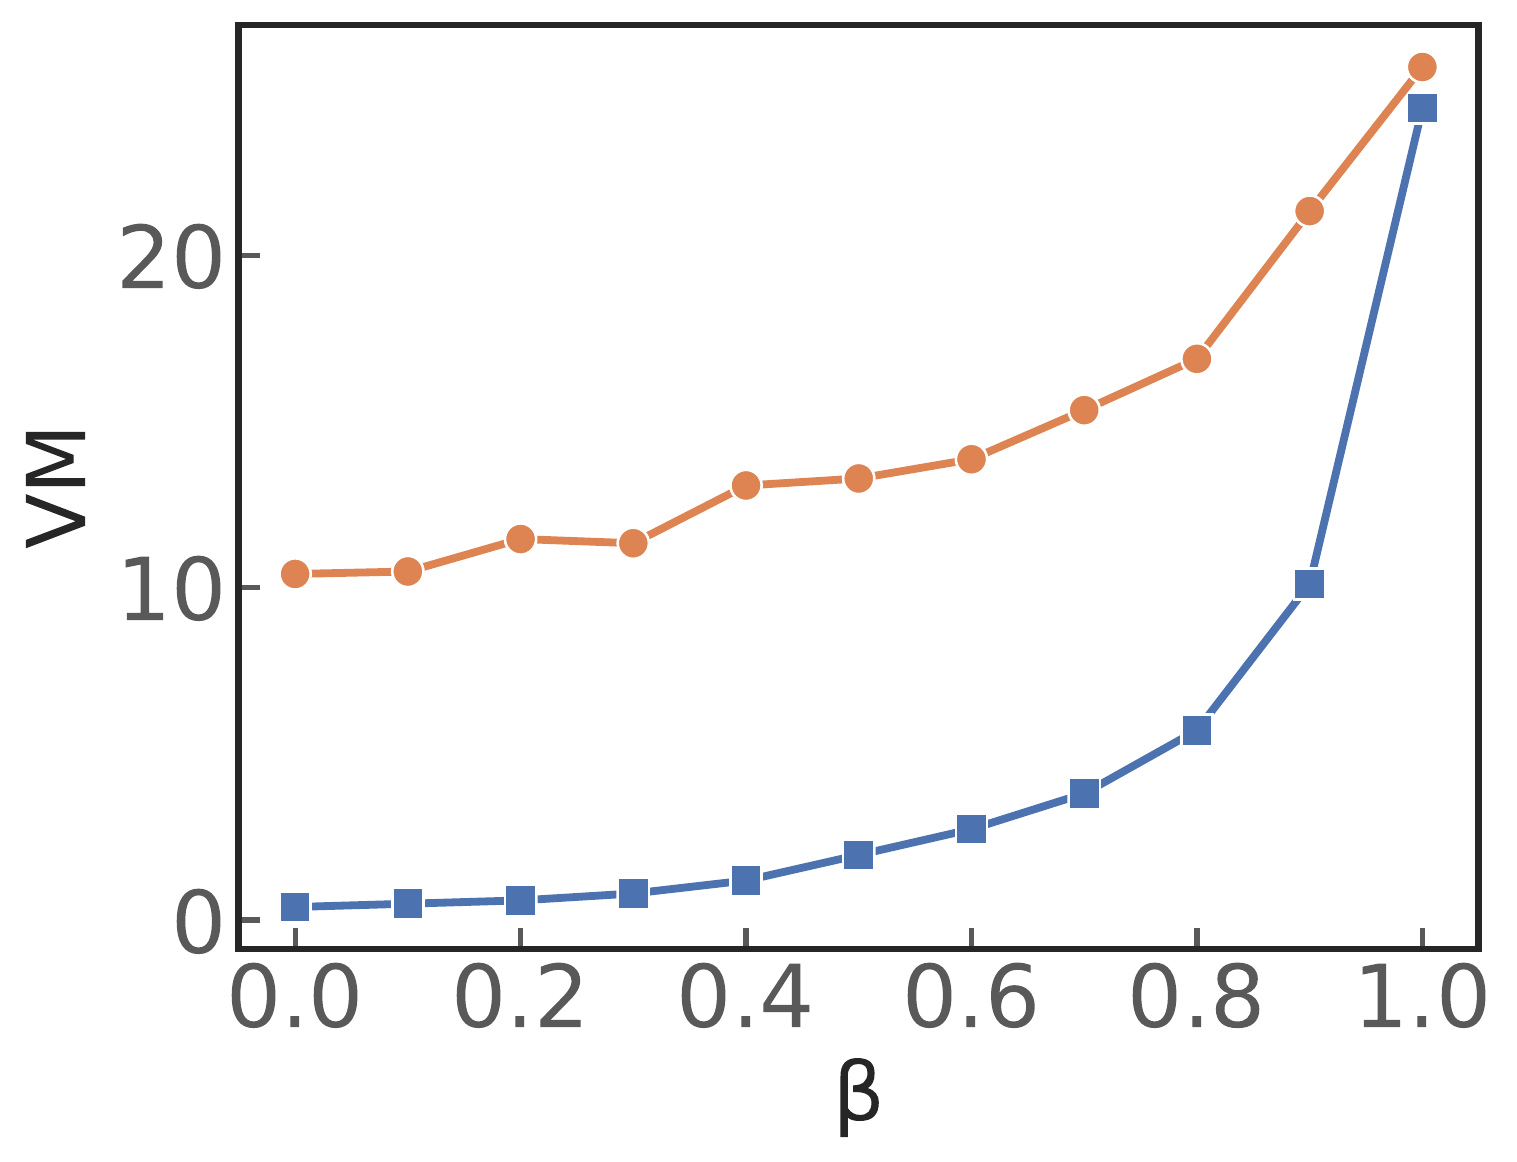}
%     \hspace{5pt}
%     \includegraphics[scale=0.3]{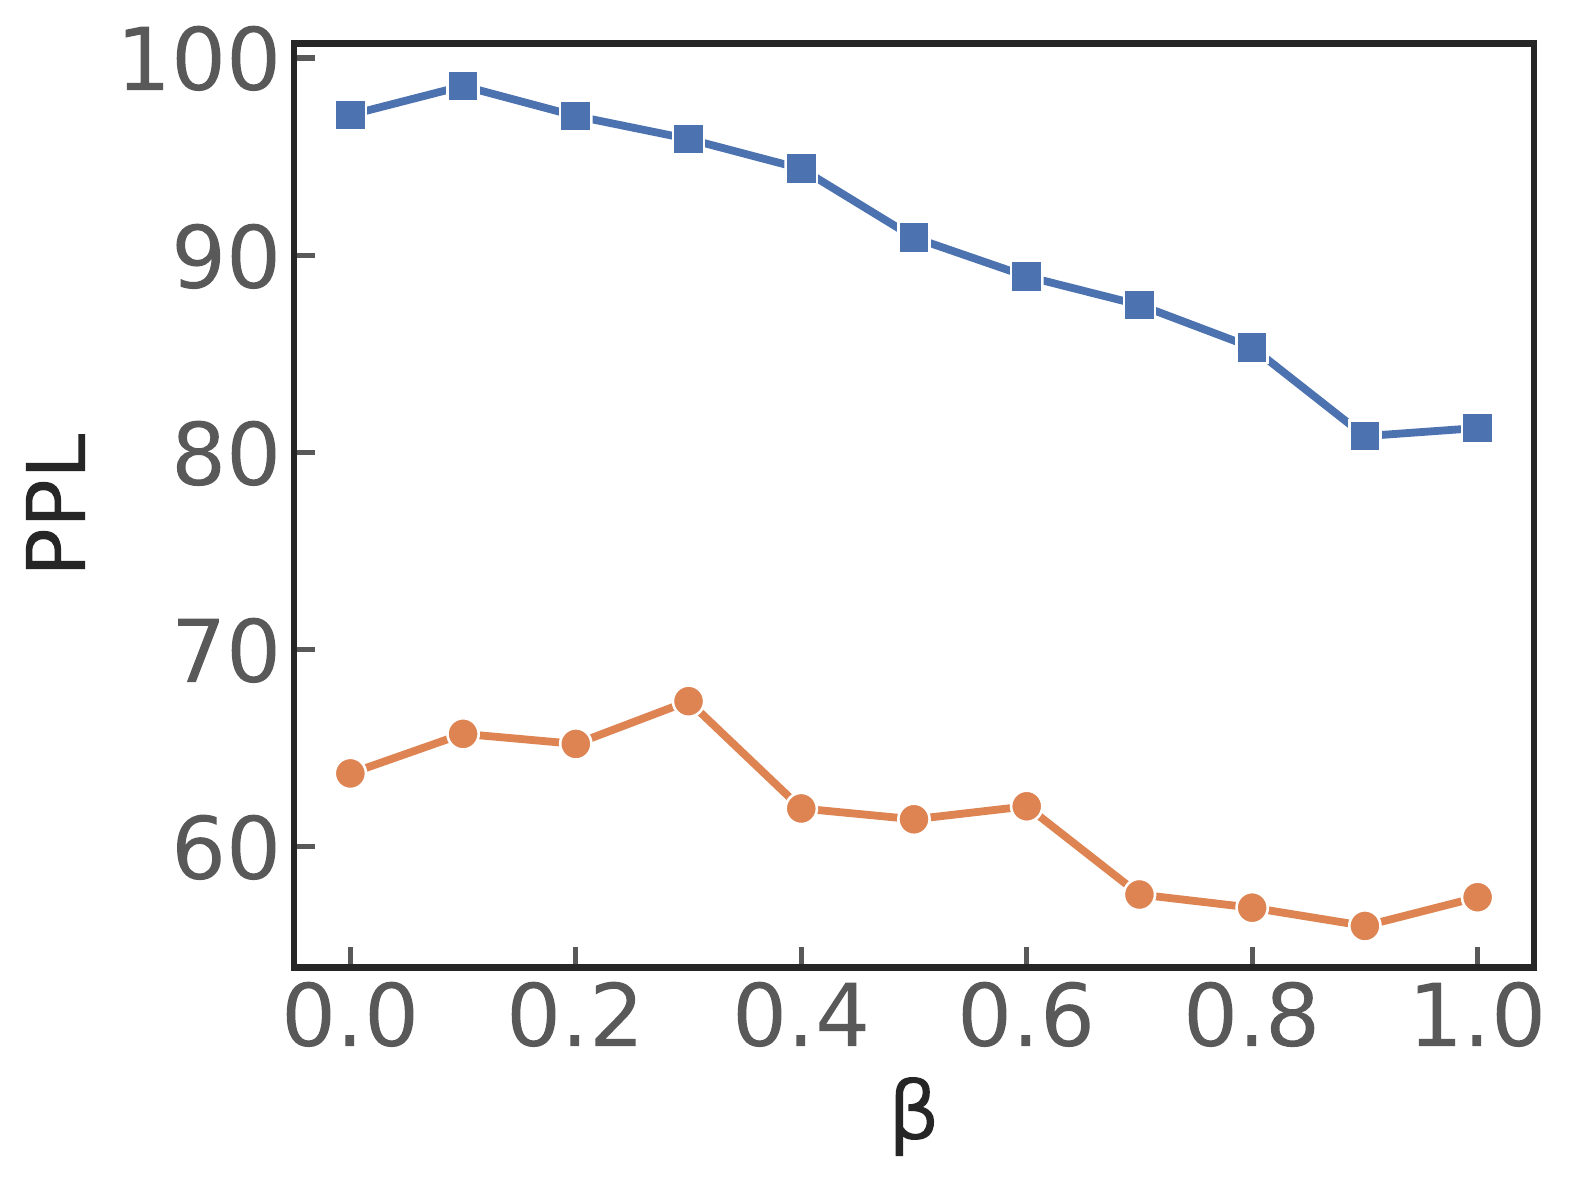}
%     % \includegraphics[scale=0.5]{naaclhlt2019-latex/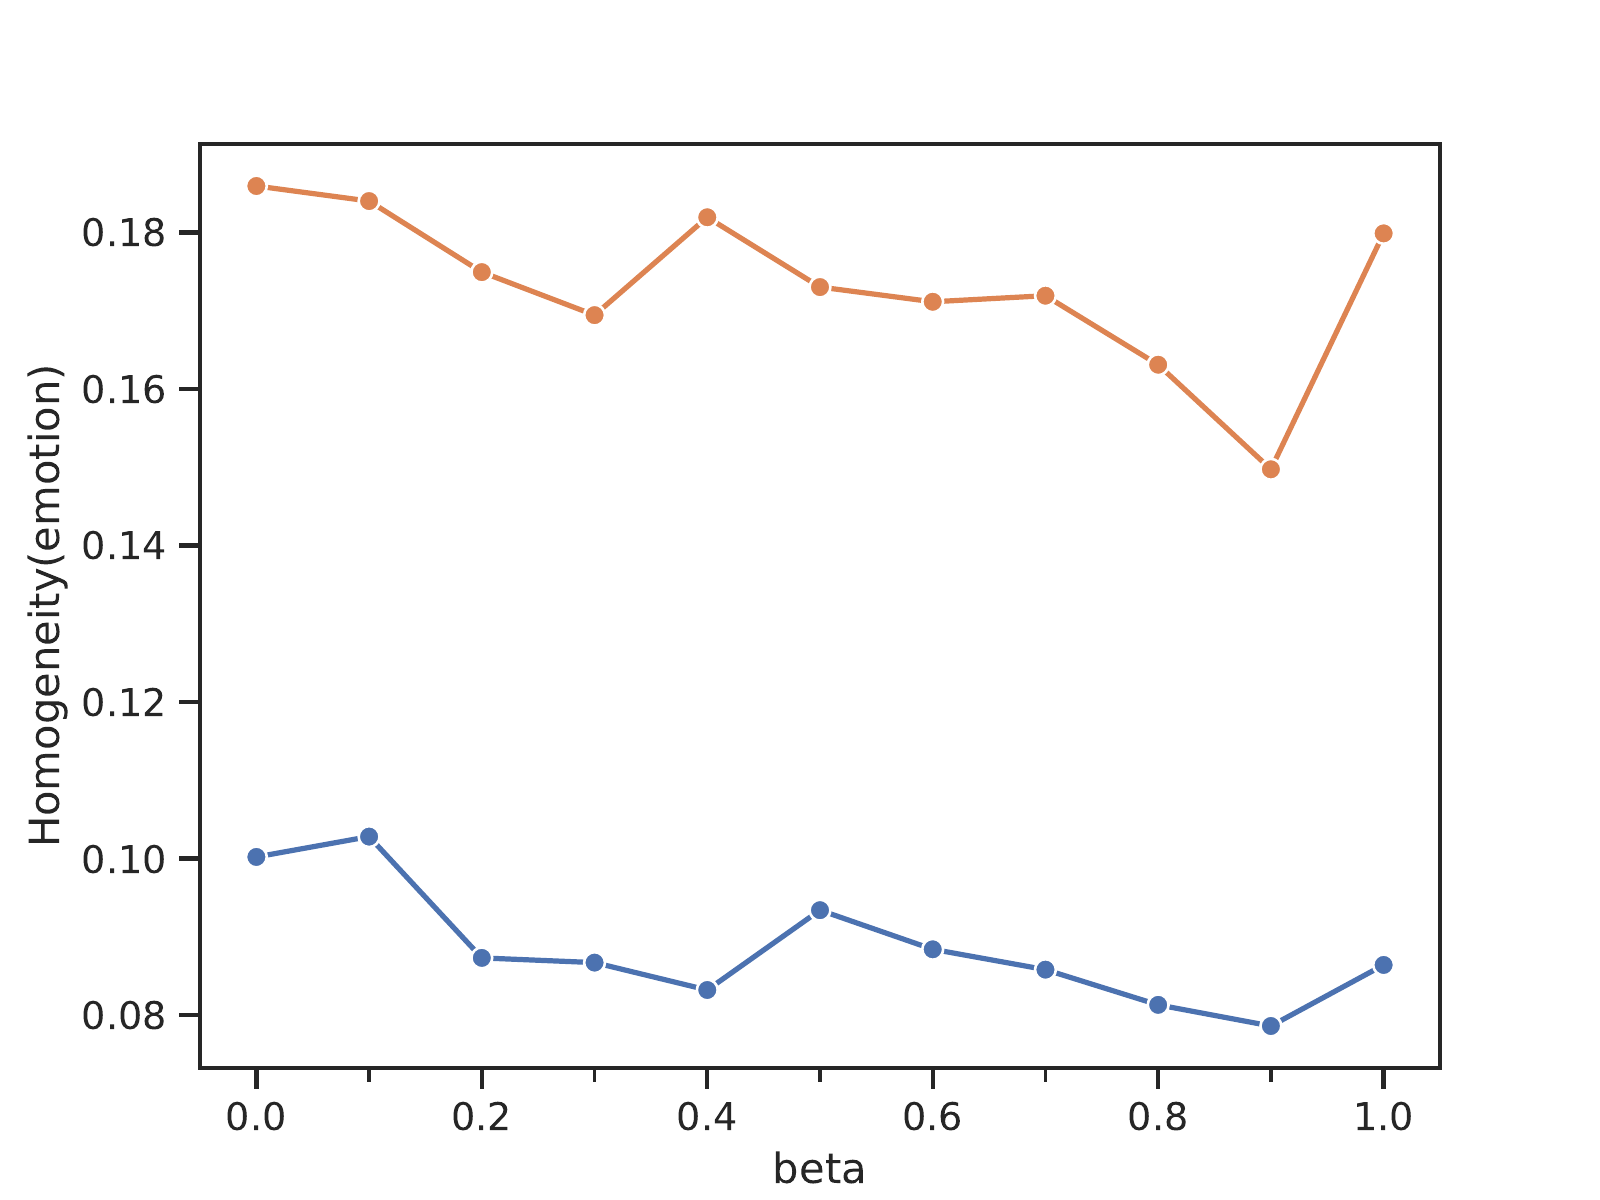}
%     % \includegraphics[scale=0.5]{naaclhlt2019-latex/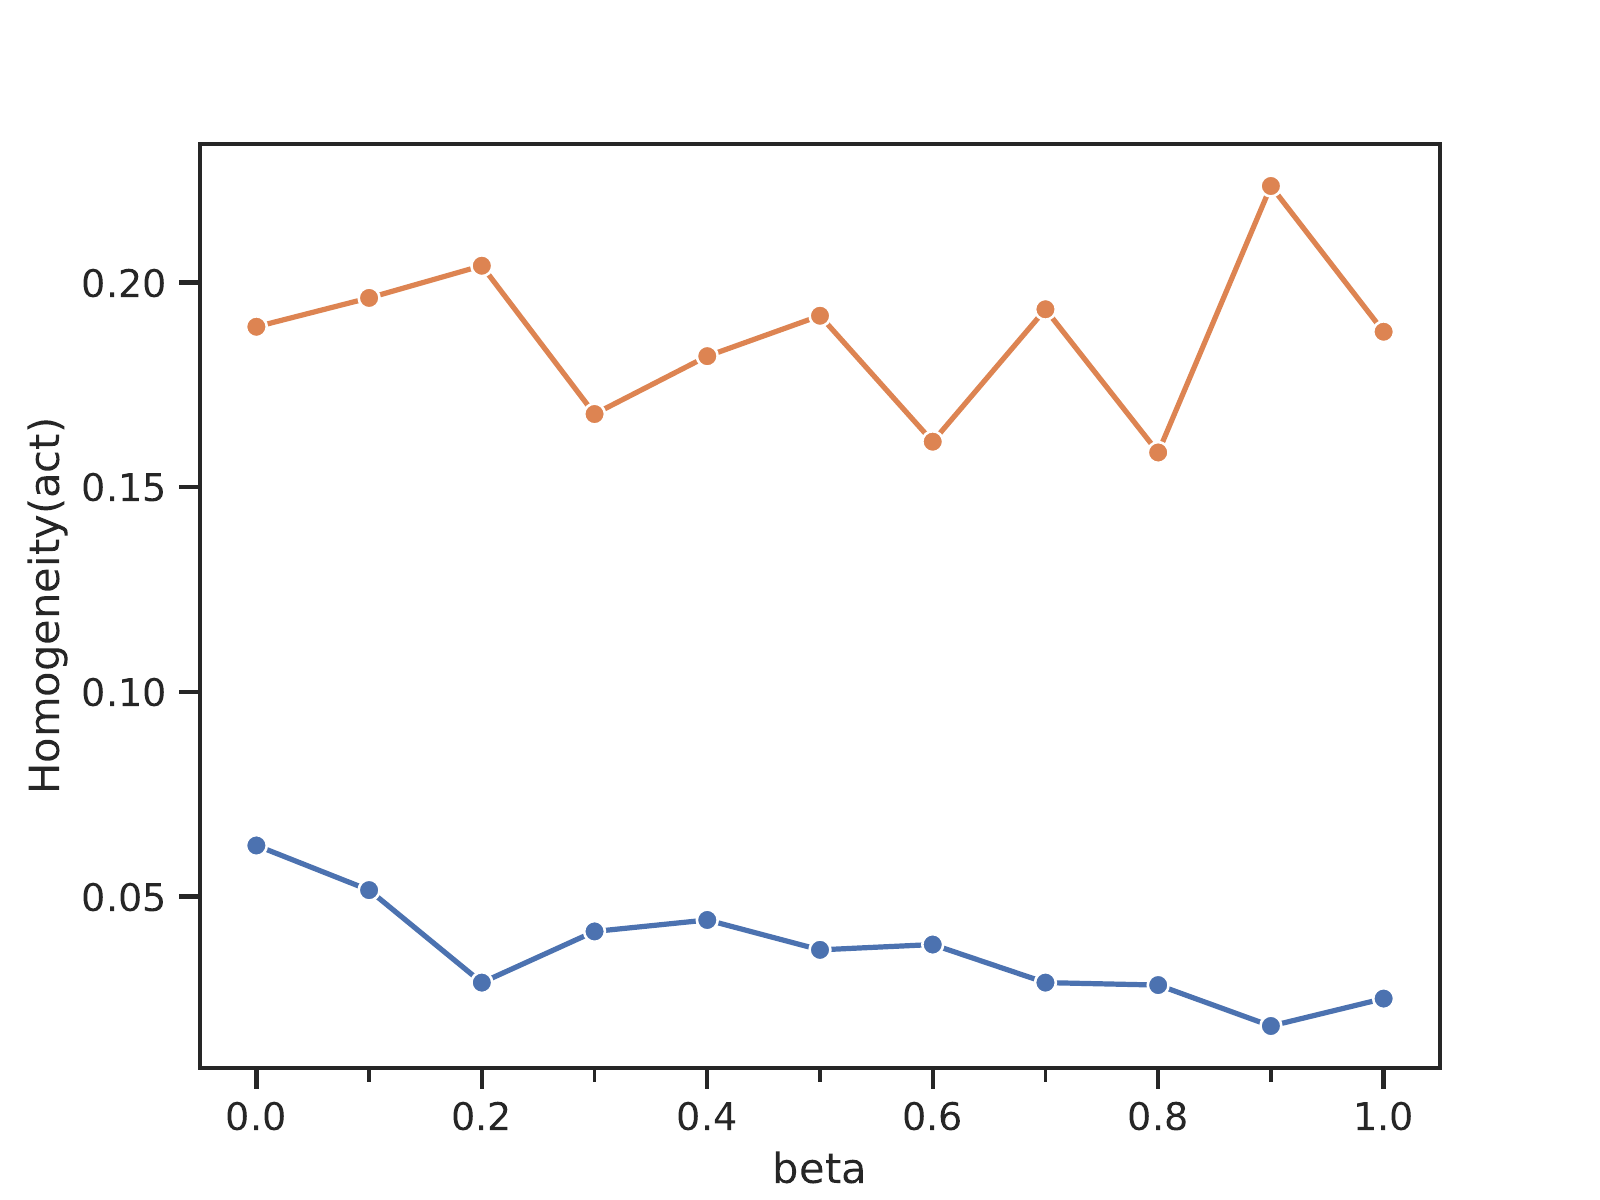}
%     \caption{VM and PPL of \methodshort with different $\beta$, on the validation set of PTB. Results of \methodshort $-$ $\LL_{\text{mi}}$ and \methodshort are displayed by the blue lines and orange lines, respectively.}
%     \label{fig:ptb_beta}
% \end{figure}

\section{More Cases}
More examples of actions discovered by \methodshort is shown in Tab.~\ref{tab:more-case-actions}. More examples on responses generated by \methodshort are shown in Tab.~\ref{tab:more-case-response}. In Tab.~\ref{tab:more-case-response}, an example without context is given to show the ability to begin a dialog in different topics (weather, navigation and scheduling). For \methodshort, we can sample different continuous latent variables from one component. As shown in Tab.~\ref{tab:more-case-response-from-c}, diverse responses with the same actions could be generated.

\begin{table*}[htb]
\centering
\small
% \begin{tabular}{cc}
\begin{tabular}{l|l}
\hline
{\bf Action Name} & Request-location \\
\hline
{\bf Utterances} & Which location do you want the weather for? \\
% & There is a Chevron 3 miles away. \\
& Which location should I look up information about? \\
% & There is a Philz 6 miles away. \\
& Which city are you asking about? \\
\hline
\hline
{\bf Action Name} & Inform-time/appointment \\
\hline
{\bf Utterances} & Your next dinner event is with your father on Friday. \\
% & What is the forecast in my city? \\
& Your father will be attending your yoga activity on the 2nd with you. \\
& Your doctor's appointment is Monday at 1 pm. \\
% & What is the weather like today in tomorrow? \\
\hline
\hline
{\bf Action Name} & General-thanks \\
\hline
{\bf Utterances} & Thanks. \\
% & What is the forecast in my city? \\
& Thanks a lot. \\
& Perfect. Thanks. \\

\hline
% \end{tabular}
\end{tabular}
\caption{Example actions discovered by \methodshort on SMD. The action name is annotated by experts.  }\label{tab:more-case-actions} % discovered by \methodshort
\end{table*}

\begin{table*}[htb]
\centering
\small
\begin{tabular}{l|l}
\hline
% {\bf Context} & \textit{User:} What gas stations are here?  \\
% & \textit{Sys:} There is a Chevron. \\
{\bf Context} & \textit{User:} What's the temperature going to be this week? \\
& \textit{Sys:} What city are you wanting to know the temperature for?\\
\hline
{\bf Predict} & (1-1-0, inform-address) Cleveland. \\
& (4-0-2, request-weather) Will it rain in Redwood City today? \\
\hline
\hline
{\bf Context} & None \\
\hline
{\bf Predict} & (1-4-0, request-route/address) find me a nearby coffee shop \\
& (1-0-4, request-weather) what's the weather going to be like today and tomorrow   \\
& (1-2-4, command-reminder) remind me about meeting later \\
\hline
\end{tabular}
\caption{Dialog cases on SMD, which are generated by sampling different $c$ from policy network. The label of sampled $c$ are listed in parentheses with the annotated action name. When context is None, it means to predict the beginning a dialog.}\label{tab:more-case-response}
\end{table*}

\begin{table*}[htb]
\centering
\small
\begin{tabular}{l|l}
\hline
% {\bf Context} & \textit{User:} What gas stations are here?  \\
% & \textit{Sys:} There is a Chevron. \\
{\bf Context} & \textit{User:} What is the highest temperature in Brentwood  over the next two days? \\
\hline
{\bf Action Name} & (2-3-0) inform-weather \\
\hline
{\bf Predict} & It is currently foggy in Brentwood on Tuesday.  \\
% & It will be warm in Redwood City right now. \\
& It will be between 70 - 40F and turn - 40F on Saturday. \\
\hline
\hline
{\bf Context} & \textit{User:} I need gas. \\
\hline
{\bf Action Name} & (2-4-2) inform-route/address \\
\hline
{\bf Predict} & There is a Chevron 3 miles from you.\\
& There is a Safeway.  \\
% & It will be between 70 - 40F and turn - 40F on Saturday. \\
\hline
\hline
{\bf Context} & \textit{User:} schedule meeting \\
\hline
{\bf Action Name} & (3-0-4) request-time \\
\hline
{\bf Predict} & What day and time should I set your meeting for? \\
& What time should I set the alarm?  \\
\hline
\end{tabular}
\caption{Dialog cases on SMD, which are generated by sampling different $z$ from the same actions (i.e., the $c$). }\label{tab:more-case-response-from-c}
\end{table*}
